# Supplementary material for: UniMark: Artificial Intelligence Generated Content Identification Toolkit
Source: arXiv:2512.12324 source file (2026-04-02)
Supplement: Supplementary file 1 [file Appendices.tex]

\begin{appendices}

    \end{appendices}
